# Supplementary material for: Strong interactions between dipolar polaritons
Source: arXiv:1804.04975 ancillary file (2018-04-13)
Supplement: Supplementary file 1 [file Dipolariton_supplementary_note.pdf]

# Supplementary Note 1. DETAILED INFORMATION ON THE SAMPLE STRUCTURE AND FABRICATION

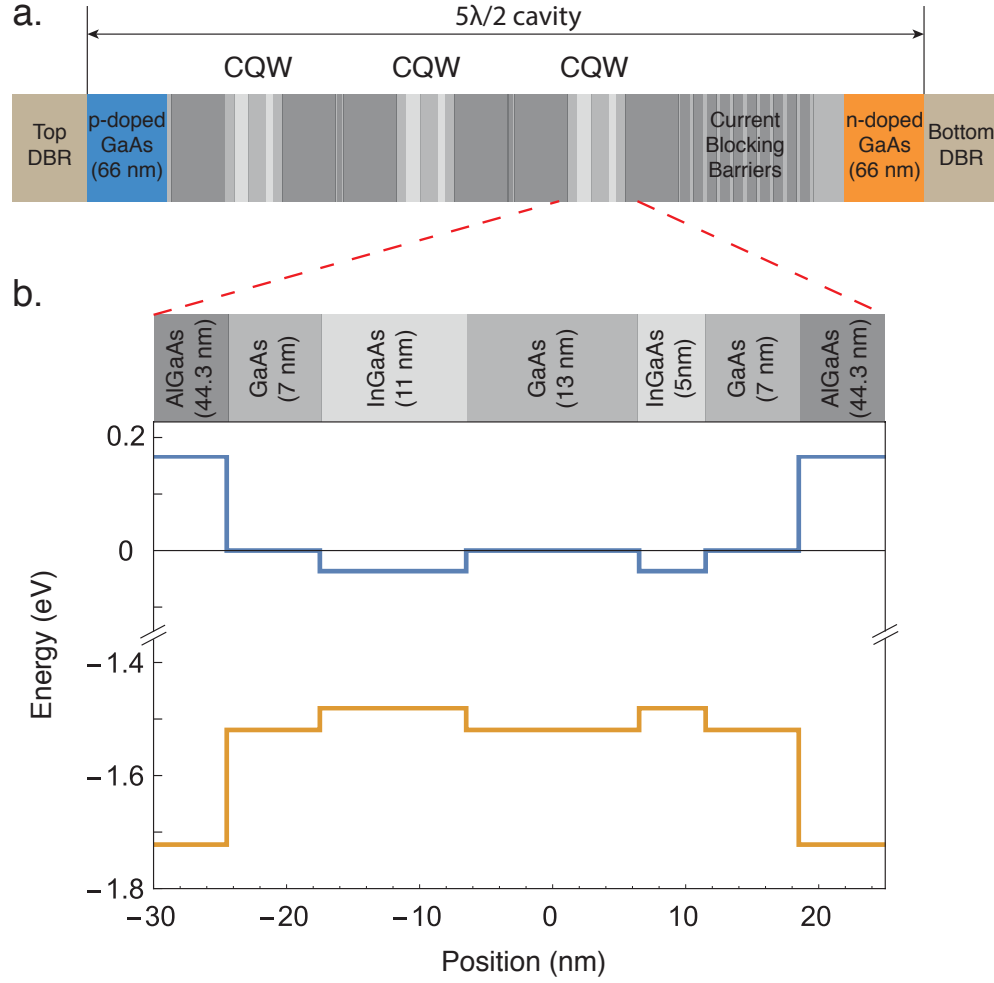

Supplementary Figure 1: **Sample structure in the growth direction and corresponding band diagram at electric field  $E = 0$ .** **a.** The sample structure between the two distributed Bragg reflector (DBR) mirrors contain  $p$  (carbon as dopant) and  $n$  (silicon as dopant) doped layers, a current blocking barrier, and three repetitions of a structure that contains a pair of QWs. The current blocking layer consists of 10 repetitions of a GaAs (3.3 nm)/Al<sub>0.23</sub>Ga<sub>0.77</sub>As (7.7 nm) superlattice structure. The tunnel barriers are Al<sub>0.23</sub>Ga<sub>0.77</sub>As. **b.** The blue line is the conduction band diagram of electrons and the orange line is the valence band diagram of heavy holes at  $E = 0$ .

As shown in Supplementary Figure 1, the two quantum wells in the coupled quantum well (QW) structure have different thicknesses, one is 11 nm thick and the other is 5 nm thick. This is to ensure that the direct and indirect exciton energies will be on resonance at finite electric field.

In the absence of the an electric field  $E$ , indirect exciton (IX) energy  $\epsilon_{IX}$  is larger than the direct exciton (DX) energy  $\epsilon_{DX}$ . As  $E$  increases,  $\epsilon_{IX}$  decreases linearly with  $E$  due to the permanent dipole moment of IX, whereas  $\epsilon_{DX}$  decreases more slowly (quadratically) with  $E$ . With this difference in the well thicknesses, only at some finite electric field the condition  $\epsilon_{IX} \sim \epsilon_{DX}$  is satisfied. Thus by tuning the electric field we can control the detuning between the exciton states, and bring them into resonance.

During the molecular beam epitaxy growth of our sample, the growth temperature of most GaAs layers was 610 °C. During the growth of the distributed Bragg reflectors (DBRs), the temperature was increased to 625 °C and for the InGaAs layers it was reduced to 480 °C. After the growth of each QW, it was capped with 5 nm GaAs grown at the same temperature before heating to 610 °C during a growth interruption. These growth temperatures were measured with a pyrometer.

We use standard photolithography, wet etching, metal deposition and rapid thermal annealing techniques to make Ohmic contacts to the  $p$  and  $n$  doped layers. To expose the  $p$  and  $n$  doped regions around the contact areas, we use a selective wet etch of GaAs followed by a selective wet etch of AlAs to remove each layer that forms the top DBR. A solution of 4:1 citric acid to hydrogen peroxide is used for selective etching of GaAs layers, and 3:1:50 ratio of phosphoric acid, hydrogen peroxide to water is used for selective etching of AlAs layers. To make an Ohmic contact to the  $n$  doped layer, following the removal of the top DBR layer, we remove the  $p$  doped layer in a 3:3:100 mixture of sulfuric acid, hydrogen peroxide to water [1]. On the exposed surface we deposit 52.8/107.2/52.8/107.2/80/100 nm of Ge/Au/Ge/Au/Ni/Au. The sample is then annealed at 400 °C for 30 seconds. To make an Ohmic contact to the  $p$  doped layer we deposit 15/10/15/60 nm of Pt/Ti/Pt/Au in a region where the top DBR has been etched and anneal the sample for 30 seconds at 300 °C.

## Supplementary Note 2. EXTRACTION OF $g_P$ FROM REFLECTION DATA

Within the standard input-output formalism, the expectation value of the photon field output from the polariton system can be written as :

$$a_{\text{out}} = a_{\text{in}} + c\sqrt{\gamma_{\text{in}}}p = \sqrt{I^{\text{in}}} + c\sqrt{\gamma_{\text{in}}}p,$$

where  $p$  denotes the polariton annihilation operator,  $\gamma_{\text{in}}$  the input coupling rate,  $c$  is the generalized Hopfield coefficient of the cavity mode of polaritons, and  $I^{\text{in}}$  is the input intensity. The quantity

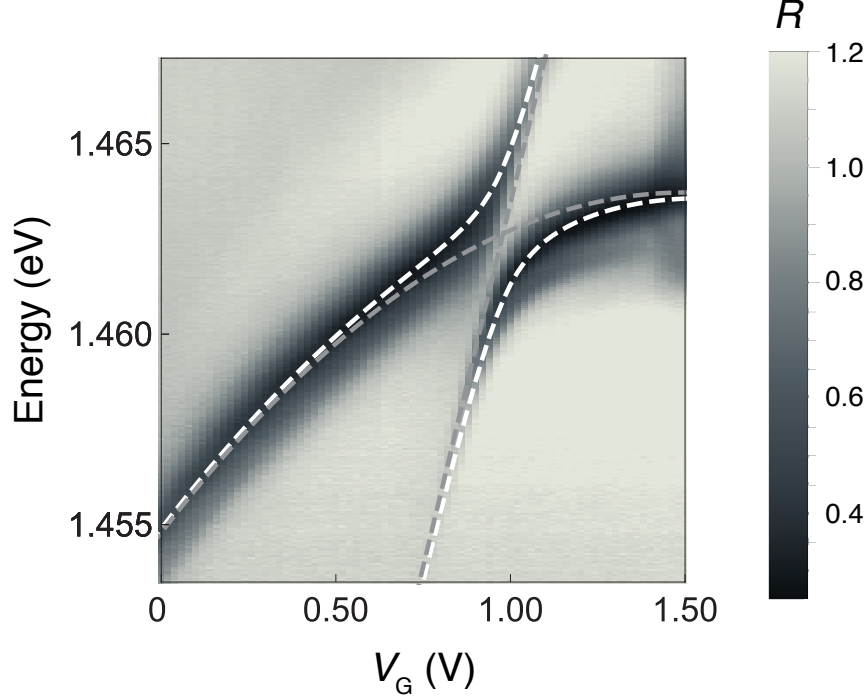

Supplementary Figure 2: **Reflection spectrum of exciton energy with respect to gate voltage  $V_G$ .**

The normalized spectrum is measured at a point where the top DBR has been etched, hence features on the spectrum are solely due to the QW exciton resonances in our sample. Resonances of direct exciton (DX) and indirect exciton (IX) show anti-crossing at  $V_G \sim 0.98$  V (at finite electric field). Gray dashed lines shows uncoupled DX and IX energies, and white dashed lines correspond to DX-IX coupled eigenenergies calculated as the eigenvalues of the matrix in Eq. 1 in main text, with  $\Omega = 0$ . Electron tunneling strength of  $J = 3.5$  meV matches well with the measured data. On our sample, the relation between the applied electric field  $E$  and the gate voltage  $V_G$  is given by  $E = (1.5 - V_G)/l$ , where  $l = 550$  nm is the distance between  $p$  and  $n$  metal gates.

measured in reflection spectra is:

$$|a_{\text{out}}|^2 / I^{\text{in}}.$$

The quantity measured in differential reflection is modelled as:

$$dR = A \left( I^{\text{in}} - |a_{\text{out}}|^2 \right) + B, \quad (\text{S1})$$

where  $A$  is a proportionality constant based on the detector gain, collection efficiency, etc and  $B$  is due to changes in the background noise of the detector, room lights, etc. We use the steady state solution of Eq. 2 to obtain  $p$  in the expressions above. Except for  $g_P$  all values of the

parameters in Eq. 2 can be measured independently, and we use the mean measured (low power) value of  $\gamma_P = 103 \mu\text{eV}$ , the value of  $c$  extracted from Eq. 1 for each position and gate voltage, and the measured power value for  $I^{\text{in}}$ . We assume  $\gamma_{\text{in}}$  does not change in our sample, and we use  $\gamma_{\text{in}} = \gamma_P/6 \sim 17 \mu\text{eV}$ , to match the measured reflection spectra (see also Supplementary Note 6). For each  $dR$  trace, obtained at a given position and gate voltage, we fit Eq. S1 to identify values of  $g_P$  and  $B$ . The proportionality constant  $A$  is fixed to match the  $dR$  trace with the model given in Eq. S1 at  $V_G = 1.4 \text{ V}$  with  $|x|^2 = 0.24$  and  $|y|^2 = 0.002$ . Finally we note that  $dR \propto |p|^2$  is a good approximation to the data that we have obtained, see Supplementary Figure 3.

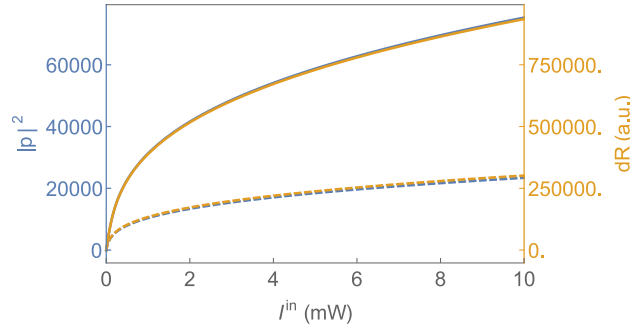

Supplementary Figure 3: **Simulated polariton population vs  $dR$ .** We show the simulated polariton number  $|p|^2$  on the left axis (blue traces), and  $dR$  calculated using Eq. S1 with  $A = 1$  and  $B = 0$  on the right axis (yellow traces) as a function of laser power  $I^{\text{in}}$  for  $g_P = 20 \text{ neV}$ ,  $|c|^2 = 0.7$  (solid lines, corresponding to  $V_G = 1.1 \text{ V}$  in Figure 4) and  $g_P = 100 \text{ neV}$ ,  $|c|^2 = 0.5$  (dashed lines, corresponding to  $V_G = 0.95 \text{ V}$  in Figure 4). Note that  $dR \propto |p|^2$ . We will treat the experimental  $dR$  signal to be unitless for the rest of the text.

### Supplementary Note 3. EXPERIMENTAL DETAILS

#### A. Determination of polariton resonance

For all experiments that are based on resonant laser excitation we employ a pulse sequence to reduce effects of laser induced slow changes to the polariton transition frequencies. At each position and gate voltage we determine the unperturbed lower polariton resonance energy ( $\epsilon_{\text{LP}}$ ) and linewidth ( $\gamma_P$ ) by measuring the reflected intensity of a weak laser as its energy is scanned across the resonance. The laser's intensity is chosen to be low enough so it does not perturb the transition energy of the polariton resonance. This laser is modulated using a waveguide amplitude modulator (EOSpace AZ-0K5-10-PFA-PFAP-950-, we denote as EOM in figures) to produce rect-

angular pulses with an on duration of  $2.5 \mu\text{s}$  and peak intensity of  $\sim 400 \text{ nW}$ , that is repeated at a period of  $10 \text{ ms}$ . This excitation is linearly polarized on the sample and at each laser energy we measure the reflected intensity as a function of time  $R(V_G, t)$ . For any target gate voltage  $V_G$  we perform a second measurement at  $0 \text{ V}$ , at this second voltage the excitation laser is not resonant with polariton transitions. The voltage applied to the sample is switched between these values following a few hundred periods of the pulse sequence ( $\sim 5 \text{ s}$ ). To obtain the normalized reflection at a particular laser energy ( $\epsilon_L$ ) we calculate the average change in the reflected intensity  $\langle R(V_G, t, \epsilon_L)/R(0 \text{ V}, t, \epsilon_L) \rangle$  where the average is taken over the on time of the pulse.

### B. Differential reflection measurement

To measure effects of changing the power of an excitation laser on the excited polariton number we tune a second laser to the energy  $\epsilon_{LP}$ . We use an AOM (single-pass, extinction ratio  $\leq 40 \text{ dB}$ ) to modulate the intensity of this second laser to produce a single sinusoidal pulse that is typically  $250 \text{ ns}$  long, again repeated at a period of  $10 \text{ ms}$  as shown in Supplementary Figure 4a. Note that  $2.5 \mu\text{m}$  weak laser pulse is blocked in this measurement. When measuring differential reflection we, again, record the time trace of the light reflected from the sample,  $R(V_G, t)$ , for a target  $V_G$  where the laser energy coincides with polariton resonance as well as at  $0 \text{ V}$  where laser energy is not resonant with polariton mode so that all the incident light is reflected. To obtain the differential reflection signal (See the red dashed line of Figure 2b for example) we calculate the difference between the two time traces obtained  $dR(t) = R(0 \text{ V}, t) - R(V_G, t)$ . Note that at certain time  $t'$  of the time traces the incident laser's intensities are identical to both  $R(0 \text{ V}, t')$  and  $R(V_G, t')$ . Hence,  $dR(t)$  signals measured at different time correspond to the data with measured at different applied laser powers. Hence we can assign the mean intensity of the excitation laser to a time interval to obtain plots of differential reflection to input power.

### C. Effect of slow dynamics on polariton resonance

In order to ensure that the applied strong laser pulse does not lead to significant changes in the polariton transition frequency on a timescale that is much longer than the polariton lifetime, we carry out two laser experiments to measure the shift of the polariton resonance. To this end we monitor the reflection spectrum of the weak laser before, during, and after the  $250 \text{ ns}$  pulse. The pulse sequence used for these experiments is illustrated in Supplementary Figure 5a, and is a

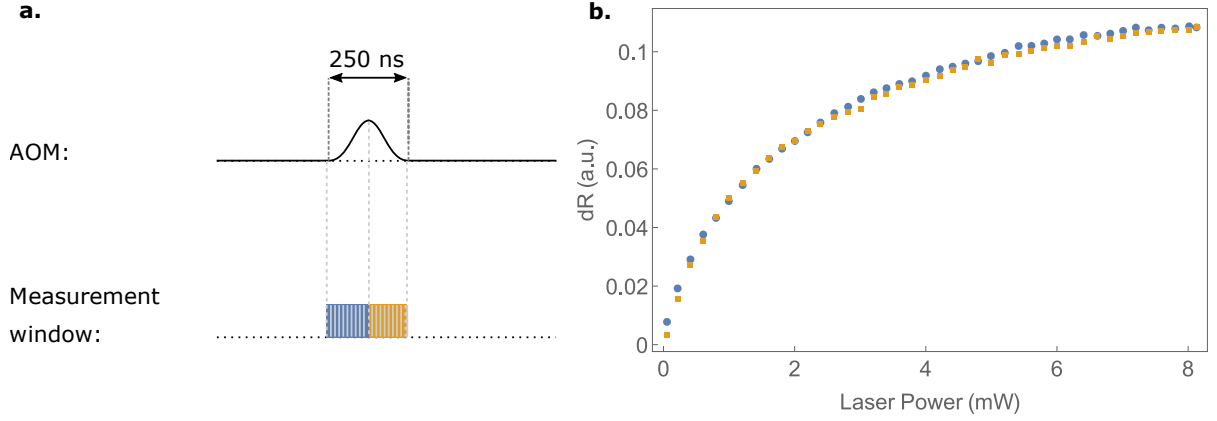

Supplementary Figure 4: **Pulse sequence used in experiments where  $dR$  is measured and results of such experiments at  $V_G = 1.1$  V.** **a.** The strong laser is modulated with an AOM so that it has a sinusoidal pulse shape. A The pulse sequence is repeated with a period 10 ms. Measurement of the reflection trace as a function of time for each laser energy allows us to define measurement windows that correspond to intervals during the rising edge of the sinusoidal pulse (blue), and during the falling edge of the sinusoidal pulse (yellow). **b.** Results  $dR$  measurements during the rising and falling edge of the sinusoidal pulse, at  $V_G = 1.1$ . Blue curve is what was used in Figure 2b.

combination of the two experiments described earlier. The two excitation lasers are orthogonally linearly polarized when exciting the sample, hence by setting the angle of the polarizer in front of the collection optics for measuring the reflection signal we can selectively suppress the laser whose intensity is varied. The reflection spectrum obtained in these two laser experiments is calculated by  $[R(V_G, t, \epsilon_L) - R_{rf}(t)] / R(0 \text{ V}, t, \epsilon_L)$ , where we subtract a value  $R_{rf}$  that is due to the resonance fluorescence of polaritons polarized orthogonal to the laser whose intensity is varied. Since  $R_{rf}$  does not change with the energy of the weak laser we can identify its value when the weak laser is off resonant with the polariton transition ( $\epsilon'_L$ : bluest  $N$  datapoints,  $N$  typically 5)  $R_{rf}(t) = \frac{1}{N} \left[ \sum_{\epsilon'_L} R(V_G, t, \epsilon'_L) - R(0 \text{ V}, t, \epsilon'_L) \right]$ . We then post-select a particular time window to obtain different reflection spectra before the pulse (blue), at the peak of the pulse (yellow), and after the pulse (green), see Supplementary Figure 5a. We identify the polariton resonance for these three time windows and to quantify the shift of the polariton resonance from the unperturbed state we pick the polariton resonance energy before the 250 ns pulse ( $\epsilon_{P,b}$ ) and denote the shift as  $\Delta_b = \epsilon_{LP} - \epsilon_{P,b}$  as shown in Supplementary Figure 5b. This shift of the polariton resonance energy when the strong laser has negligible intensity has important implications to the accuracy with which we can determine  $g_P$ , we discuss these in Supplementary Notes 4 and 5.

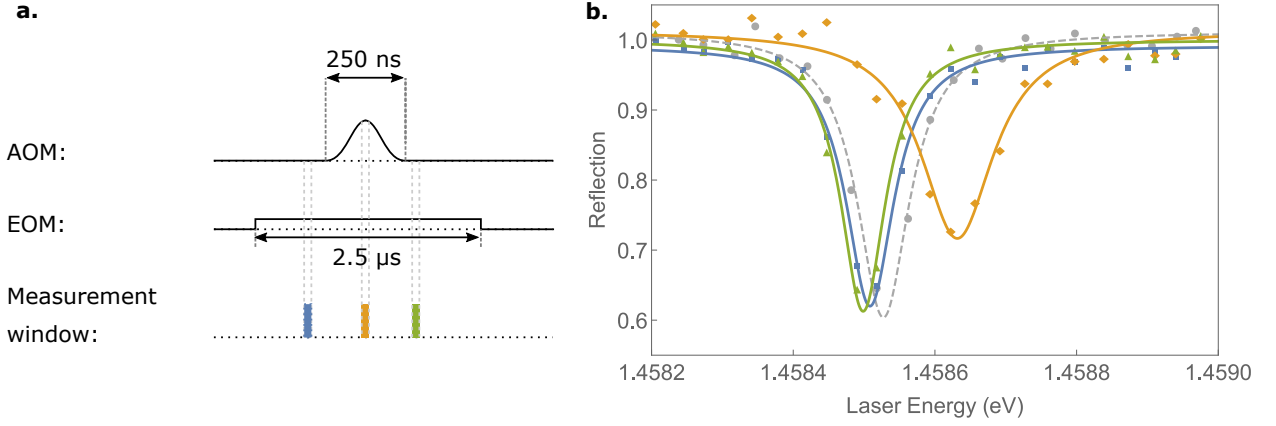

Supplementary Figure 5: **Pulse sequence used in experiments where the blue-shift of the polariton resonance is measured as a function of applied laser power and results of such experiments at  $V_G = 1.1$  V.**

**a.** The strong laser is modulated with an AOM so that it has a sinusoidal pulse shape. A waveguide based amplitude modulator is used to modulate a weak laser to produce a rectangular pulse shape. The pulse sequence is repeated with a period 10 ms. The energy of the weak laser ( $\epsilon_L$ ) is stepped through the polariton resonance after a few hundred repetitions of the pulse sequence. Measurement of the reflection trace as a function of time for each laser energy allows us to define measurement windows that correspond to intervals before (blue), at the peak intensity of (yellow) and after (green) the sinusoidal strong laser pulse. **b.** Results of two laser experiments where the reflection spectrum 100 ns before (blue), at the peak intensity of (yellow), and 100 ns after (green) the 250 ns pulse is shown. Also on the figure is the result of the reflection experiment when the 250 ns laser pulse is blocked (gray). At  $V_G = 1.1$  V the presence of the 250 ns pulse leads to a red-shift of the resonance that decays over a slow timescale. 100 ns after the pulse we measure the resonance to be red-shifted by  $29 \mu\text{eV}$ , whereas before the pulse the red shift is  $\Delta_b = 19 \mu\text{eV}$ . We note that using this pulse sequence the effect of slow dynamics on the polariton resonance is limited to shifts that are smaller than the linewidth of the polariton resonance which is  $90 \mu\text{eV}$ .

#### Supplementary Note 4. VARIATION OF MEASURED $g_P$ DUE TO SLOW CHANGES IN THE POLARITON ENVIRONMENT

When we measure  $g_P$  using differential reflection, we measure multiple traces of  $dR$  at a given position. For example at  $V_G = 1.4$  V and  $|x|^2 = 0.24$  and negligible  $|y|^2$ , the mean of the standard deviation of the extracted values of  $g_P/g_0$  through these traces of  $dR$  is 0.013. When we repeat the experiment at different positions with the same  $|x|^2$  and  $V_G$  value, the standard deviation of the estimate of  $g_P/g_0$  is 0.21. A histogram of the measurements is shown in Supplementary Figure 6.

We believe the variation for  $g_P$  between different positions are due to differences in the polariton environment that lead to slow changes in the polariton resonance frequency (see Supplementary Note

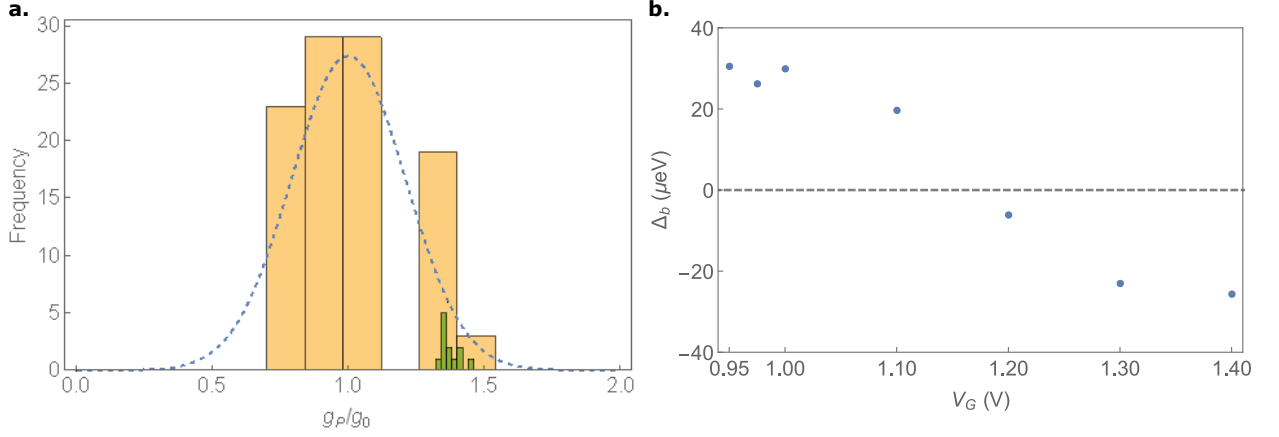

Supplementary Figure 6: **Histogram of measured  $g_P$  values at  $V_G = 1.4$  V,  $|x|^2 = 0.24$  and  $|y|^2 = 0.002$ , and measured  $\Delta_b$  values as a function of  $V_G$ .** **a.** The green chart shows the frequency of the extracted  $g_P$  for a single position on the sample. The yellow charts show the cumulative frequency of the extracted  $g_P$  for 9 different positions with equal  $|x|^2$  and  $|y|^2$  values at  $V_G = 1.4$  V. Blue dashed line shows a (scaled) normal distribution with a mean of 1 and standard deviation of 0.21. **b.** A plot of the measured  $\Delta_b$  values as a function of  $V_G$  is presented. The data is obtained at the location where we have acquired the gate voltage dependent blue-shift data that is used in Supplementary Note 5. This measurement implies our excitation laser is blue detuned from the polariton resonance for low gate voltages, and red detuned for high gate voltages, we underestimate  $g_P$  at low gate voltages, and overestimate it at high gate voltages

3). Since the laser whose intensity is varied is tuned to  $\epsilon_P$ , the shift of the polariton resonance away from its unperturbed value even at times when the strong pump laser has negligible intensity presents a detuning to Eq. 2 that is determined by the position and gate voltage, which alters the extracted  $g_P$ . We characterize this detuning with  $\Delta_b$  (see Supplementary Note 3). For example at  $V_G = 1.1$  V,  $|x|^2 = 0.29$  and  $|y|^2 = 0.01$ , we measure  $\Delta_b = 7 \pm 12 \mu\text{eV}$  in three repetitions of the two laser experiment (similar to Supplementary Figure 5) at different points on the sample with the same  $|x|^2$  and  $|y|^2$ , and the polariton FWHM linewidth to be  $90 \mu\text{eV}$ . We estimate the influence of the presence of such an uncontrolled detuning on our estimate of  $g_P$  by simulating a  $dR$  signal using Eq. 2 with  $\delta_P = -\Delta_b$  measured for 1.1 V. We then fit the simulated  $dR$  trace using the method described in Supplementary Note 2 (i.e. with  $\delta_P = 0$ ) and find that it leads to a variation of the extracted  $g_P$  by 12 %.

We also note that, at the position that we obtain the gate voltage dependent blue-shift data (see Supplementary Note 5), the measured  $\Delta_b$  changes with applied voltage. This is illustrated in Supplementary Figure 6. We estimate the detunings measured at this, different, position would

lead to an overestimation of the  $g_P$  value at 1.4 V by 15 % and an underestimation of the  $g_P$  value at 0.95 V by 15 %.

### Supplementary Note 5. EXTRACTION OF INTERACTION STRENGTH USING TWO LASER EXPERIMENTS

We use the power dependent blue-shift of the polariton resonance under the illumination of a pump laser at fixed energy to extract  $g_P$  as we vary the IX and DX contents. This is a complementary method to the differential reflection based estimates presented in the main text and discussed earlier, and relies on the blue-shift of the lower polariton resonance that was illustrated in Figure 2b. We use the same experimental sequence as described in Supplementary Note 3 and illustrated in Supplementary Figure 5, where we define non-overlapping 10 ns long time windows inside the 250 ns sinusoidal pulse to monitor the polariton resonance energy ( $\epsilon_P(I^{\text{in}})$ ) as a function of the pump power. As described in Supplementary Note 3, the presence of a pulse of the laser at energy  $\epsilon_L$  causes a change in the environment of the polaritons with a slow timescale, and shifts the polariton resonance before the pulse is applied to  $\epsilon_{P,b}$ . The reflection spectrum obtained by the energy sweep of the weak laser during the application of the pulse sequence is used to determine the blue-shift of the polariton resonance ( $\Delta_{LP} = \epsilon_P(I^{\text{in}}) - \epsilon_{P,b}$ ) as a function of the intensity of the laser at energy  $\epsilon_L$ . We note while  $dR$  is proportional to  $|p|^2$ , the blue-shift  $\Delta_{LP}$  is proportional to  $g_P|p|^2$ . Hence changes in the ratio of the  $\Delta_{LP}$  to the  $dR$  trace should also give an estimate of the relative changes to  $g_P$ . Changes in this ratio with gate voltage  $V_G$  is illustrated in Supplementary Figure 7.

The results of this complementary method of obtaining the change in  $g_P$  differs from those presented in the main text in two important ways. First the change in  $g_P$  with  $V_G$  is much more significant, we estimate roughly a factor of 10 increase of  $g_P$  from  $V_G = 1.4$  V to  $V_G = 0.95$  V. Using the  $dR$  data only the difference is roughly a factor of 5. As pointed out in Supplementary Note 4, it is likely that the our measurements of the changes in  $g_P$  using only  $dR$  underestimates the gate voltage dependent increase in  $g_P$ . Second difference is in the model that describes the change in  $g_P$ . For the method that uses both  $dR$  and  $\Delta_{LP}$  we find  $g_P = g_0a(|x|^4 + b|y|^4 + c|x|^2|y|^2)$  with  $a = 19$ ,  $b = 6$  and  $c = 2$  fits our data well, whereas for the estimate of  $g_P$  using  $dR$  data only we find  $a = 17$ ,  $b = 8$  and  $c = 0.2$  which indicates that the IX DX interactions are negligible.

With our data it is difficult to ascertain which of the two measurements is more accurate. In particular the measurement of  $\Delta_{LP}$  relies on measuring the shift of the polariton mode that

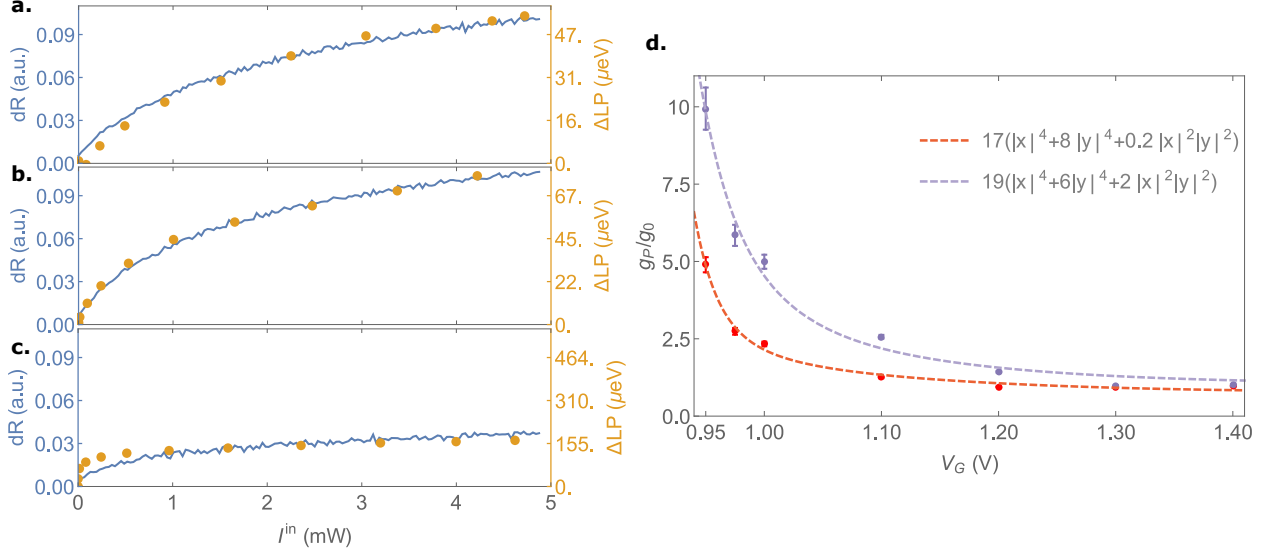

Supplementary Figure 7: **Changes of  $g_P$  measured using blue-shift of the polariton resonance.** **a-c.** Plots showing power dependent  $dR$  (left axis) and  $\Delta_{LP}$  (right axis) at different gate voltages. We use the two axis representation to show the two traces as well as to indicate the scale factor ( $\alpha$ ) that best matches  $\alpha dR = \Delta_{LP}$ , the value of  $\alpha$  is obtained from a least-squares fit. **a** is measured at  $V_G = 1.4$  V with  $\alpha = 520 \mu\text{eV}$ , **b** is measured at  $V_G = 1.2$  V with  $\alpha = 740 \mu\text{eV}$ , and **c** is measured at  $V_G = 0.95$  V with  $\alpha = 5200 \mu\text{eV}$ . **d.** Estimated changes in  $g_P$  as a function of gate voltage  $V_G$ . In purple we show the change in the ratio  $\alpha/520$ , our estimate of  $g_P/g_0$  using both the blue-shift and the reflection data. The errorbars of the purple points is the  $1 \sigma$  confidence interval of the parameter estimate obtained from the least squares fit. In red we show the data with linear polarization as shown in Figure 4 in the main text.

couples to linearly polarized light that is orthogonal to the excitation laser, and thus is not a direct measurement of the blue-shift of the polariton mode that is excited. As illustrated in Supplementary Figure 7c, we observe, an increase in  $\Delta_{LP}$  at small intensities that is not well captured by the behaviour expected from Eq. 2. This is particular to low gate voltages. Hence the increase of  $g_P$  that we report in the main text is most likely a lower estimate. Low power photon correlation measurements carried out in confined cavities [2], that should be free of the slow dynamics present in our experiments may more accurately determine the interactions between dipolar polaritons.

## Supplementary Note 6. SIMULATION OF POLARITON DYNAMICS INCLUDING A SPATIAL DEGREE OF FREEDOM

We simulate polariton dynamics including a single spatial dimension to account for effective mass of polaritons, finite spot-size of the pump beam, and changes in spatial distribution of the polariton wavefunction with pump intensity. We show that for the parameters relevant to the experiments reported in this manuscript, the single mode model used in the main text is a good approximation of the polariton dynamics. These simulations also allow us to extract  $U_{\text{DX}}$ , the DX-DX interaction constant.

We model the lower polariton behaviour by solving the following 1-dimensional (1D) mean field partial differential equation:

$$\delta_P \psi(x, t) - \frac{\hbar}{2m_P} \frac{\partial^2}{\partial x^2} \psi(x, t) + g'_P |\psi(x, t)|^2 \psi(x, t) - i \frac{\gamma_P}{2} \psi(x, t) - ic \sqrt{\gamma_{\text{in}}} A^{\text{in}}(x) = i \frac{\partial}{\partial t} \psi(x, t) \quad (\text{S2})$$

where  $\psi(x, t)$  is the mean field polariton wavefunction,  $\delta_P$  is the detuning of the laser from the polariton mode,  $\hbar$  is the reduced Planck constant,  $m_P$  is the polariton effective mass,  $g'_P$  is the nonlinear coefficient,  $\gamma_P$  is the polariton linewidth,  $c$  is the generalized Hopfield coefficient defined in the main text,  $\gamma_{\text{in}}$  characterizes the input coupling rate, and  $A^{\text{in}}$  is the driving field amplitude. We use  $\mu\text{m}$  for units of  $x$  values and  $1/m_P \sim |c|^2/m_{\text{ph}}$ , where a cavity photon mass  $m_{\text{ph}}$  is  $6 \times 10^{-5} m_e$  where  $m_e$  is the free electron mass [3]. Following [4]:  $g'_P = U_P/(4.25 \mu\text{m})$  where  $4.25 \mu\text{m}$  is our estimate of the FWHM of our pump spot. We solve the PDE with boundary conditions  $\psi(\pm 100, t) = 0$  till  $t = 10/\gamma_P$ . We use  $A^{\text{in}}(x) = A^{\text{in}} e^{-\frac{x^2}{4\sigma^2}}$  where  $A^{\text{in}} = \sqrt{I^{\text{in}}/(\sigma\sqrt{2\pi})^2}$  where  $\sigma = 4.25/2.35 \mu\text{m}$ ,  $I^{\text{in}}$  is the input power, a normalization factor is included in converting the input power to the field so that the experimentally measured power corresponds to the total integrated power in the simulation. In order to compare the results of the simulation with the experimental results we calculate two quantities.

The first quantity is the simulated reflected intensity detected in the fiber coupled photodiode. We assume the spatial mode profile of light detected by the fiber coupled photodiode is the same as that of the excitation beam  $A^{\text{in}}(x)$ . Hence the simulated reflected intensity is calculated as the overlap of the pump beam with the light output from the polariton system, normalized to the pump intensity:

$$\eta \times \frac{\int |A^{\text{ref}}(x)|^2 dx}{\int |A^{\text{in}}(x)|^2 dx},$$

where  $A^{\text{ref}}(x) = A^{\text{in}}(x) + ic\sqrt{\gamma_{\text{in}}}\psi(x, 10/\gamma_{\text{P}})$  indicates the amplitude of the reflected light and  $\eta = \left| \int A^{\text{in},*}(x) A^{\text{ref}}(x) dx \right|^2 / \left( \int |A^{\text{in}}(x)|^2 dx \int |A^{\text{ref}}(x)|^2 dx \right)$  is the overlap between the reflected light and the pump beam corresponding to the portion of reflected light coupling into our single mode fiber collection mode.

We calculate the simulated reflected intensity for  $I^{\text{in}} = 1 \mu\text{W}$  and a range of detunings to obtain a simulated, low power, reflection spectrum. By comparing the simulated spectrum, in particular the linewidth and the contrast of the polariton resonance we determine,  $\gamma_{\text{P}} = 60 \mu\text{eV}$  and  $\gamma_{\text{in}} = \gamma_{\text{P}}/4 \sim 15 \mu\text{eV}$ . Note that  $\gamma_{\text{in}}$  value estimated here is similar to  $\gamma_{\text{in}}$  value ( $\sim 17 \mu\text{eV}$ ) we used in 0D simulation. Note that  $\gamma_{\text{P}}$  has contributions from loss through lower mirror, mirror losses, or non-radiative decay, etc. With these values simulations produce results in good agreement with the experimental data as shown in Supplementary Figure 8a. We note that the linewidth measured in the reflection spectrum (80 - 90  $\mu\text{eV}$ , see Figure 4c) is wider than  $\gamma_{\text{P}}$  because of the effective mass of polaritons, and finite  $k$  space width of the excitation and detection spots. Moreover the increase in the effective mass with the change in the gate voltage from  $V_{\text{G}} = 1.1 \text{ V}$  to  $0.95 \text{ V}$  leads to narrowing of the linewidth of the reflection spectrum from 90  $\mu\text{eV}$  to 82  $\mu\text{eV}$ .

The second quantity we calculate is the simulated differential reflection signal, which is given by

$$\int |A^{\text{in}}(x)|^2 dx - \eta \times \int |A^{\text{ref}}(x)|^2 dx.$$

We multiply the resulting value with a single constant factor for all our simulations to be able to compare with experimental data. We fix the detuning to  $\delta_{\text{P}} = 0$  and vary  $I^{\text{in}}$  to obtain the simulated power dependence of the differential reflection signal. With  $|c|^2 = 0.7$ ,  $g'_{\text{P}} = 50 \text{ neV } \mu\text{m}$  for  $V_{\text{G}} = 1.1 \text{ V}$ , and  $|c|^2 = 0.52$ ,  $g'_{\text{P}} = 190 \text{ neV } \mu\text{m}$  for  $V_{\text{G}} = 0.95 \text{ V}$ , we obtained reasonable agreement with our experimental data and simulation results, see Supplementary Figure 8b. Note that, these values indicate an enhancement of factor of 3.8 in  $g_{\text{P}}$  in between  $V_{\text{G}} = 0.95 \text{ V}$  and  $1.1 \text{ V}$ , and this is in good agreement with the value of 3.5 reported in Figure 4 in the main text where a single mode polariton model was used for analysis.

In Supplementary Figure 8c, we plot spatial distribution of polaritons  $|\psi(x)/\psi(0)|^2$  at  $t = 10/\gamma_{\text{P}}$ . Note that polariton spatial distribution is broader than pump profile but relative change of spatial distribution with respect to  $V_{\text{G}}$  and input power are not substantial within our experimental conditions.

Since IX content is negligible at  $V_{\text{G}} = 1.1 \text{ V}$ , we use the  $g'_{\text{P}}$  extracted at this voltage, to estimate

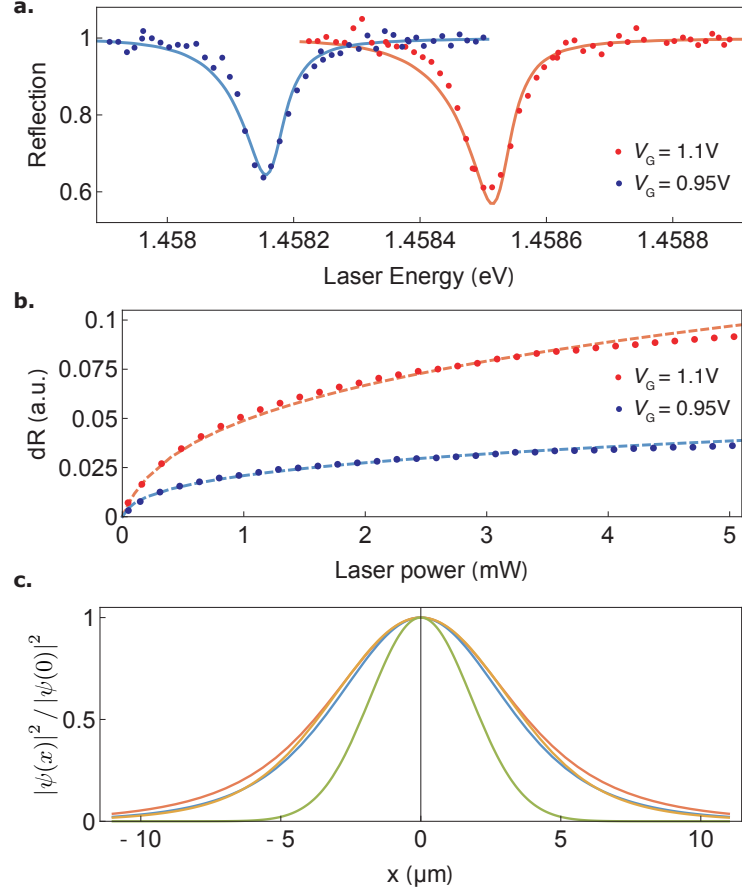

Supplementary Figure 8: **Comparison between experimental results and 1D simulations.** **a.** Experimental (dots) and simulated (solid line) reflection spectra. The experimental signal is obtained as described in Supplementary Note 3. The simulated spectra is obtained by calculating the simulated reflected intensity at  $I^{\text{in}} = 1 \mu\text{W}$  and varying the detuning  $\delta_P$ . **b.** Experimental (dots) and simulated (dashed lines) differential reflection signal. The experimental signal is obtained as described in Supplementary Note 3. The simulated signal is obtained by varying  $I^{\text{in}}$  at  $\delta_P = 0$ . **c.** 1D simulation results on spatial distributions of polaritons at  $t = 10/\gamma_P$  normalized by  $|\psi(0)|^2$ . Red, blue, and yellow lines correspond to  $V_G = 1.1 \text{ V}$  with  $I^{\text{in}} = 1 \mu\text{W}$ ,  $V_G = 0.95 \text{ V}$  with  $I^{\text{in}} = 1 \mu\text{W}$ ,  $V_G = 0.95 \text{ V}$  with  $I^{\text{in}} = 5 \text{ mW}$ , respectively. Corresponding FWHMs are  $7.6 \mu\text{m}$ ,  $7.0 \mu\text{m}$ , and  $7.4 \mu\text{m}$ . Green dashed line indicates a normalized pump intensity profile  $|A^{\text{in}}(x)/A^{\text{in}}(0)|^2$  for comparison to  $|\psi(x)/\psi(0)|^2$ .

DX-DX interaction strength  $U_{\text{DX}}$ :

$$U_{\text{DX}} = \frac{U_P}{|x|^4} = \frac{g'_P \times 4.25 \mu\text{m}}{|x|^4} \sim 2.4 \mu\text{eV} \mu\text{m}^2.$$

We note that the  $g_0$  used in the main-text is consistent with this value of  $U_{\text{DX}}$  as  $Ag_0/|x|^4 \sim 1.4 \mu\text{eV} \mu\text{m}^2$ , where we used  $A = 7^2 \mu\text{m}^2$ , based on the polariton distribution shown in Supplementary

Figure 8. Since in our sample we use three pairs of quantum wells and for our estimates we used linear polarization of light, we expect that the measured DX-DX interaction strength to be smaller than an estimate of the exchange based interaction among direct excitons [5, 6]:  $\sim 6E_B a_B^2 \sim 6 \mu\text{eV}\cdot\mu\text{m}^2$ . The measured value is also smaller compared to recent measurements of the DX interaction strength ( $30 \mu\text{eV}\cdot\mu\text{m}^2$ ) with microcavity polaritons with a single InGaAs QW [7]. Note that since we do not really have an independent method of measuring the pump spot size that we assume or the photon mass that we use, the extracted values have an intrinsic uncertainty. Hence, we think that the estimated interaction strength can easily differ by factor of two.

Since our system is 2D and we convert some of the parameters assuming a spatial length in the perpendicular dimension (for example in terms of how the input power is normalized and  $g'_P$  is normalized) our estimates can be improved by carrying out 2D simulations.

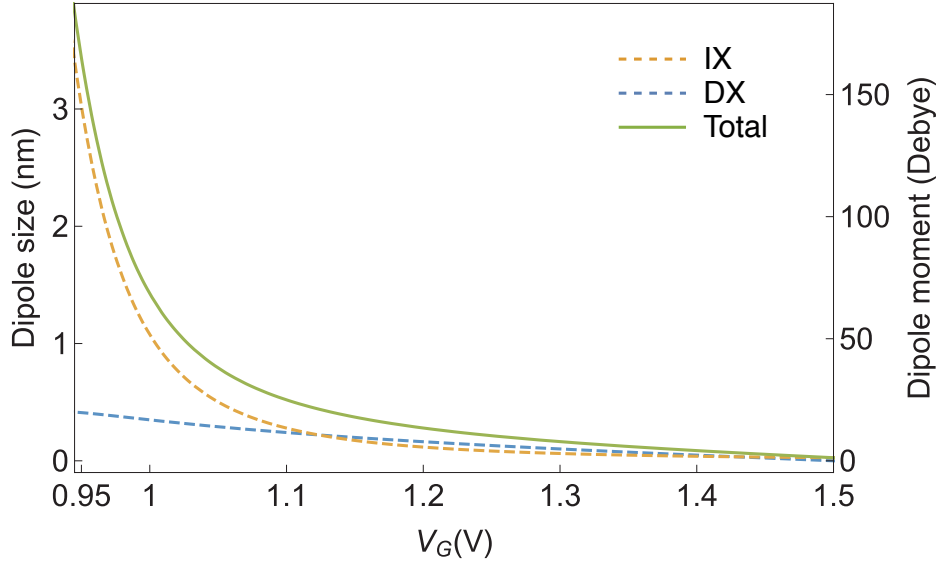

Supplementary Figure 9: **Effective dipole size of the lower polariton with respect to  $V_G$ .** This is the estimated effective dipole size of the lower polariton for the sample position where the data of Figure 4 in the main text was taken. For IXs, the size of the dipole is  $d = 21$  nm, while the induced dipole moment of DXs is proportional to the electric field  $E$ . Hence, the effective dipole moment of the lower polariton is given by  $d_{\text{eff}} = \alpha E |x|^2 + e d |y|^2$ , where  $\alpha$  is the polarizability of the DX and  $e$  is the elementary charge. Orange dashed line is the dipole size due to IX contribution while blue dashed line is the dipole size contribution from DX content. Green solid line is the total effective dipole size of the lower polariton.

- 
- [1] M. Grska, H. Wrzesiska, J. Muszalski, J. Ratajczak, and B. Mroziejewicz, *Materials Science in Semiconductor Processing* **5**, 505 (2002), ISSN 1369-8001, URL <http://www.sciencedirect.com/science/article/pii/S1369800102000719>.
  - [2] G. Muoz-Matutano, A. Wood, M. Johnson, X. V. Asensio, B. Baragiola, A. Reinhard, A. Lemaitre, J. Bloch, A. Amo, B. Besga, et al., arXiv:1712.05551 [cond-mat] (2017), arXiv: 1712.05551, URL <http://arxiv.org/abs/1712.05551>.
  - [3] H.-T. Lim, E. Togan, M. Kroner, J. Miguel-Sanchez, and A. Imamolu, *Nature Communications* **8**, 14540 (2017), ISSN 2041-1723, URL <http://www.nature.com/doifinder/10.1038/ncomms14540>.
  - [4] E. Wertz, A. Amo, D. D. Solnyshkov, L. Ferrier, T. C. H. Liew, D. Sanvitto, P. Senellart, I. Sagnes, A. Lematre, A. V. Kavokin, et al., *Physical Review Letters* **109** (2012), ISSN 0031-9007, 1079-7114, URL <https://link.aps.org/doi/10.1103/PhysRevLett.109.216404>.
  - [5] C. Ciuti, V. Savona, C. Piermarocchi, A. Quattropani, and P. Schwendimann, *Physical Review B* **58**, 7926 (1998), URL <https://journals.aps.org/prb/abstract/10.1103/PhysRevB.58.7926>.
  - [6] F. Tassone and Y. Yamamoto, *Physical Review B* **59**, 10830 (1999), URL <https://journals.aps.org/prb/abstract/10.1103/PhysRevB.59.10830>.
  - [7] S. R. K. Rodriguez, A. Amo, I. Sagnes, L. L. Gratiet, E. Galopin, A. Lematre, and J. Bloch, *Nature Communications* **7**, ncomms11887 (2016), ISSN 2041-1723, URL <https://www.nature.com/articles/ncomms11887>.
